# Supplementary material for: Structural and magnetic properties of the quasicrystal approximant Au$_{65}$Ga$_{21}$Tb$_{14}$
Source: arXiv:2204.00868 source file (2022-04-02)
Supplement: Supplementary file 1 [file suppl_v1.pdf]

# Supplemental information on Structural and magnetic properties of the quasicrystal approximant $Au_{65}Ga_{21}Tb_{14}$

Kazuhiro Nawa, Daisuke Okuyama, Ryo Murasaki, and Taku J Sato
*Institute of Multidisciplinary Research for Advanced Materials,*
*Tohoku University, 2-1-1 Katahira, Aoba-ku, Sendai 980-8577 Japan*

Maxim Avdeev
*Australian Centre for Neutron Scattering, Australian Nuclear Science and Technology Organisation,*
*New Illawarra Rd, Lucas Heights, NSW 2234, Australia and*
*School of Chemistry, The University of Sydney, Sydney, NSW 2006, Australia*

Asuka Ishikawa
*Research Institute for Science and Technology, Tokyo University of Science, Tokyo 125-8585, Japan*

Hiroyuki Takakura
*Faculty of Engineering, Hokkaido University, Sapporo, Hokkaido 060-8628, Japan*

Chin-Wei Wang
*National Synchrotron Radiation Research Center, Hsinchu 30076, Taiwan and*
*Australian Centre for Neutron Scattering, Australian Nuclear Science and Technology Organisation,*
*New Illawarra Rd, Lucas Heights, NSW 2234, Australia*

Ryuji Tamura
*Department of Materials Science and Technology,*
*Tokyo University of Science, Tokyo 125-8585, Japan*

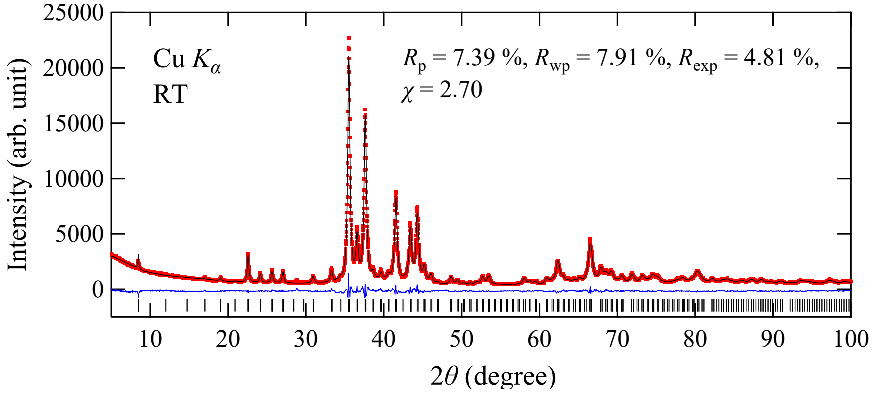


FIG. S1. Powder X-ray diffraction pattern collected at room temperature. Observed intensities, calculated intensities, and their difference are represented by red dots, black and blue curves, respectively. The position of the nuclear reflections are indicated by black solid lines.

TABLE S1. Refined crystallographic data of the powder neutron diffraction experiments.

| | 3 K (NPD) | 20 K (NPD) | 293 K (XRD) |
|---|---|---|---|
| $a$ (Å) | 14.6742(3) | 14.6737(4) | 14.7361(11) |
| $V$ (Å$^3$) | 3159.8(2) | 3159.5(3) | 3200.0(7) |
| $C_1$ ($\mu_B$) | 7.04(12) | – | – |
| $C_2$ ($\mu_B$) | −3.49(17) | – | – |
| Density (g/cm$^3$) | 15.16 | 15.16 | 14.97 |
| No. of parameters[a] | 38 | 36 | 43 |
| $2\theta$ range used for refinement (°) | 9.0–160.0 | 9.0–160.0 | 5.0–28.6, 29.0–100.0 |
| No. of nuclear reflections | 177 | 177 | 322 |
| No. of magnetic reflections | 1716 | – | – |
| $R_p$ (%) | 36.40 | 49.70 | 7.39 |
| $R_{wp}$ (%) | 25.50 | 28.50 | 7.91 |
| $R_e$ (%) | 21.23 | 23.71 | 4.81 |
| $\chi^2$ | 1.44 | 1.45 | 2.70 |
| $R_{mag}$ | 18.7 | – | – |

[a] Shift parameters are not included since they are not refined in the final refinement.

TABLE S2. Structure parameters of $Au_{65}Ga_{21}Tb_{14}$ at 3 K determined from the neutron powder diffraction experiment. The space group is $Im\overline{3}$, and the lattice parameter is $a$ = 14.6742(3). The atomic coordination is represented by a fractional coordinate. The isotropic displacement parameters $B_{iso}$ are listed in a unit of Å$^2$. Occupancy of every site and the atomic coordinate of the site with small occupancy site are fixed to those estimated from single crystalline XRD experiments.

| atom | site | $x$ | $y$ | $z$ | occupancy | $B_{iso}$ |
|---|---|---|---|---|---|---|
| Au1 | 48$e$ | 0.1034(7) | 0.3441(6) | 0.2024(6) | 1 | 0.10 |
| Ga2 | 24$e$ | 0 | 0.2344(10) | 0.0866(10) | 0.513 | 0.10 |
| Au2 | 24$e$ | 0 | 0.2344(10) | 0.0866(10) | 0.487 | 0.10 |
| Au3 | 24$e$ | 0 | 0.4024(8) | 0.3602(8) | 1 | 0.10 |
| Au4 | 16$e$ | 0.1522(7) | 0.1522(7) | 0.1522(7) | 1 | 0.10 |
| Ga5 | 12$e$ | 0.1910(13) | 0 | 0.5 | 1 | 0.10 |
| Au6 | 12$e$ | 0.4031(10) | 0 | 0 | 0.97 | 0.10 |
| Tb1 | 24$e$ | 0 | 0.1867(6) | 0.3055(6) | 1 | 0.10 |
| Ga8 | 8$e$ | 0.25 | 0.25 | 0.25 | 1 | 0.10 |
| Au7A | 24$e$ | 0 | 0.0674 | 0.0806 | 0.162 | 0.10 |
| Ga7B | 24$e$ | 0 | 0.0891 | 0.0464 | 0.087 | 0.10 |
| Tb2 | 2e | 0 | 0 | 0 | 0.026 | 0.10 |

TABLE S3. Structure parameters of $Au_{65}Ga_{21}Tb_{14}$ at 20 K determined from the neutron powder diffraction experiment. The space group is $Im\overline{3}$, and the lattice parameter is $a$ = 14.6737(4). The atomic coordination is represented by a fractional coordinate. The isotropic displacement parameters $B_{\mathrm{iso}}$ are listed in a unit of Å$^2$. Occupancy of every site and the atomic coordinate of the site with small occupancy site are fixed to those estimated from single crystalline XRD experiments.

| atom | site | $x$ | $y$ | $z$ | occupancy | $B_{\mathrm{iso}}$ |
|---|---|---|---|---|---|---|
| Au1 | 48$e$ | 0.1026(7) | 0.3441(6) | 0.2006(7) | 1 | 0.10 |
| Ga2 | 24$e$ | 0 | 0.2349(10) | 0.0844(10) | 0.513 | 0.10 |
| Au2 | 24$e$ | 0 | 0.2349(10) | 0.0844(10) | 0.487 | 0.10 |
| Au3 | 24$e$ | 0 | 0.4017(8) | 0.3568(8) | 1 | 0.10 |
| Au4 | 16$e$ | 0.1529(7) | 0.1529(7) | 0.1529(7) | 1 | 0.10 |
| Ga5 | 12$e$ | 0.1941(13) | 0 | 0.5 | 1 | 0.10 |
| Au6 | 12$e$ | 0.4000(10) | 0 | 0 | 0.97 | 0.10 |
| Tb1 | 24$e$ | 0 | 0.1856(8) | 0.3076(8) | 1 | 0.10 |
| Ga8 | 8$e$ | 0.25 | 0.25 | 0.25 | 1 | 0.10 |
| Au7A | 24$e$ | 0 | 0.0674 | 0.0806 | 0.162 | 0.10 |
| Ga7B | 24$e$ | 0 | 0.0891 | 0.0464 | 0.087 | 0.10 |
| Tb2 | 2$e$ | 0 | 0 | 0 | 0.026 | 0.10 |

TABLE S4. Structure parameters of $Au_{65}Ga_{21}Tb_{14}$ at 293 K determined from the X-ray powder diffraction experiment. The space group is $Im\overline{3}$, and the lattice parameter is $a$ = 14.7361(11). The atomic coordination is represented by a fractional coordinate. The isotropic displacement parameters $B_{\mathrm{iso}}$ are listed in a unit of Å$^2$. Occupancy of every site and the atomic coordinate of the site with small occupancy are fixed to those estimated from single crystalline XRD experiments.

| atom | site | $x$ | $y$ | $z$ | occupancy | $B_{\mathrm{iso}}$ |
|---|---|---|---|---|---|---|
| Au1A | 48e | 0.1119(6) | 0.3449(7) | 0.2085(6) | 0.36 | 1.08(6) |
| Au1B | 48e | 0.1006(3) | 0.3405(4) | 0.1960(3) | 0.64 | 1.08(6) |
| Ga2 | 24e | 0 | 0.2183(11) | 0.0938(13) | 0.513 | 0.47(11) |
| Au2 | 24e | 0 | 0.2456(5) | 0.0810(4) | 0.487 | 0.47(11) |
| Au3 | 24e | 0 | 0.4031(2) | 0.3519(2) | 1 | 1.50(6) |
| Au4 | 16e | 0.14849(14) | 0.14849(14) | 0.14849(14) | 1 | 2.50(8) |
| Ga5 | 12e | 0.1908(6) | 0 | 0.5 | 1 | 2.52(17) |
| Au6A | 12e | 0.4152(12) | 0 | 0 | 0.43 | 1.41(22) |
| Au6B | 24e | 0 | 0.3962(11) | 0.0086(20) | 0.27 | 1.41(22) |
| Tb1 | 24e | 0 | 0.1865(2) | 0.3043(3) | 1 | 1.58(6) |
| Ga8 | 8e | 0.25 | 0.25 | 0.25 | 1 | 6.05(53) |
| Au7A | 24e | 0 | 0.0674 | 0.0806 | 0.162 | 3.95 |
| Ga7B | 24e | 0 | 0.0891 | 0.0464 | 0.087 | 1.11 |
| Tb2 | 2e | 0 | 0 | 0 | 0.026 | 2.37 |

TABLE S5. List of basis vectors of all the irreducible representations for the Tb1 site in with the space group $Im\overline{3}$ and the magnetic modulation vector of $\mathbf{k}$ = (1,1,1). The Tb1 is defined to be the atomic site listed in Table. S1, such as (0, 0.1856, 0.3076). The rest of the Tb sites follow the definition given in Table. **??**. The number in parentheses represents a dimension of each IR. $\epsilon$ represents $(1+\sqrt{(3)}/2i)$.

| IRs | Tb1 | Tb2 | Tb3 | Tb4 | Tb5 | Tb6 | Tb7 | Tb8 | Tb9 | Tb10 | T11 | Tb12 |
|---|---|---|---|---|---|---|---|---|---|---|---|---|
| IR1 (1) | 1 0 0 | −1 0 0 | −1 0 0 | 1 0 0 | 0 1 0 | 0 −1 0 | 0 −1 0 | 0 1 0 | 0 0 1 | 0 0 −1 | 0 0 −1 | 0 0 1 |
| IR2-1 (1) | 0 1 0 | 0 −1 0 | 0 1 0 | 0 −1 0 | 0 0 1 | 0 0 −1 | 0 0 1 | 0 0 −1 | 1 0 0 | −1 0 0 | 1 0 0 | −1 0 0 |
| IR2-2 (1) | 0 0 1 | 0 0 1 | 0 0 −1 | 0 0 −1 | 1 0 0 | 1 0 0 | −1 0 0 | −1 0 0 | 0 1 0 | 0 1 0 | 0 −1 0 | 0 −1 0 |
| IR3 (1) | 1 0 0 | −1 0 0 | −1 0 0 | 1 0 0 | $0\ {-\epsilon}\ 0$ | $0\ \epsilon\ 0$ | $0\ \epsilon\ 0$ | $0\ {-\epsilon}\ 0$ | $0\ 0\ {-\epsilon^*}$ | $0\ 0\ \epsilon^*$ | $0\ 0\ \epsilon^*$ | $0\ 0\ {-\epsilon^*}$ |
| IR4-1 (1) | 0 1 0 | 0 −1 0 | 0 1 0 | 0 −1 0 | $0\ 0\ {-\epsilon}$ | $0\ 0\ \epsilon$ | $0\ 0\ \text{-}\epsilon$ | $0\ 0\ \epsilon$ | $-\epsilon^*\ 0\ 0$ | $\epsilon^*\ 0\ 0$ | $-\epsilon^*\ 0\ 0$ | $-\epsilon^*\ 0\ 0$ |
| IR4-2 (1) | 0 0 1 | 0 0 1 | 0 0 −1 | 0 0 −1 | $-\epsilon\ 0\ 0$ | $-\epsilon\ 0\ 0$ | $\epsilon\ 0\ 0$ | $\epsilon\ 0\ 0$ | $0\ {-\epsilon^*}\ 0$ | $0\ {-\epsilon^*}\ 0$ | $\epsilon^*\ 0\ 0$ | $\epsilon^*\ 0\ 0$ |
| IR5-1 (1) | 1 0 0 | −1 0 0 | −1 0 0 | 1 0 0 | $0\ {-\epsilon^*}\ 0$ | $0\ \epsilon^*\ 0$ | $0\ \epsilon^*\ 0$ | $0\ {-\epsilon^*}\ 0$ | $0\ 0\ {-\epsilon}$ | $0\ 0\ \epsilon$ | $0\ 0\ \epsilon$ | $0\ 0\ {-\epsilon}$ |
| IR6-1 (1) | 0 1 0 | 0 −1 0 | 0 1 0 | 0 −1 0 | $0\ 0\ {-\epsilon^*}$ | $0\ 0\ \epsilon^*$ | $0\ 0\ \text{-}\epsilon^*$ | $0\ 0\ \epsilon^*$ | $-\epsilon\ 0\ 0$ | $\epsilon\ 0\ 0$ | $-\epsilon\ 0\ 0$ | $-\epsilon\ 0\ 0$ |
| IR6-2 (1) | 0 0 1 | 0 0 1 | 0 0 −1 | 0 0 −1 | $-\epsilon^*\ 0\ 0$ | $-\epsilon^*\ 0\ 0$ | $\epsilon^*\ 0\ 0$ | $\epsilon^*\ 0\ 0$ | $0\ {-\epsilon}\ 0$ | $0\ {-\epsilon}\ 0$ | $\epsilon\ 0\ 0$ | $\epsilon\ 0\ 0$ |
| IR7-1 (3) | 1 0 0 | −1 0 0 | 1 0 0 | −1 0 0 | 0 0 0 | 0 0 0 | 0 0 0 | 0 0 0 | 0 0 0 | 0 0 0 | 0 0 0 | 0 0 0 |
| | 0 0 0 | 0 0 0 | 0 0 0 | 0 0 0 | 0 0 0 | 0 0 0 | 0 0 0 | 0 0 0 | 1 0 0 | 1 0 0 | −1 0 0 | −1 0 0 |
| | 0 0 0 | 0 0 0 | 0 0 0 | 0 0 0 | 0 0 0 | 0 0 0 | 0 0 0 | 0 0 0 | 0 1 0 | 0 −1 0 | 0 1 0 | 0 −1 0 |
| IR7-2 (3) | 0 0 0 | 0 0 0 | 0 0 0 | 0 0 0 | 0 1 0 | 0 1 0 | 0 −1 0 | 0 −1 0 | 0 0 0 | 0 0 0 | 0 0 0 | 0 0 0 |
| | 0 0 0 | 0 0 0 | 0 0 0 | 0 0 0 | 0 1 0 | 0 −1 0 | 0 1 0 | 0 −1 0 | 0 0 0 | 0 0 0 | 0 0 0 | 0 0 0 |
| | 0 1 0 | 0 1 0 | 0 −1 0 | 0 −1 0 | 0 0 0 | 0 0 0 | 0 0 0 | 0 0 0 | 0 0 0 | 0 0 0 | 0 0 0 | 0 0 0 |
| IR7-3 (3) | 0 0 1 | 0 0 −1 | 0 0 1 | 0 0 −1 | 0 0 0 | 0 0 0 | 0 0 0 | 0 0 0 | 0 0 0 | 0 0 0 | 0 0 0 | 0 0 0 |
| | 0 0 0 | 0 0 0 | 0 0 0 | 0 0 0 | 0 0 0 | 0 0 0 | 0 0 0 | 0 0 0 | 0 0 1 | 0 0 1 | 0 0 −1 | 0 0 −1 |
| | 0 0 0 | 0 0 0 | 0 0 0 | 0 0 0 | 0 0 0 | 0 0 0 | 0 0 0 | 0 0 0 | 0 0 1 | 0 0 −1 | 0 0 1 | 0 0 −1 |
| IR7-4 (3) | 0 0 0 | 0 0 0 | 0 0 0 | 0 0 0 | 0 0 1 0 | 0 0 1 | 0 0 −1 | 0 0 −1 | 0 0 0 | 0 0 0 | 0 0 0 | 0 0 0 |
| | 0 0 0 | 0 0 0 | 0 0 0 | 0 0 0 | 1 0 0 | −1 0 0 | 1 0 0 | −1 0 0 | 0 0 0 | 0 0 0 | 0 0 0 | 0 0 0 |
| | 1 0 0 | 1 0 0 | −1 0 0 | −1 0 0 | 0 0 0 | 0 0 0 | 0 0 0 | 0 0 0 | 0 0 0 | 0 0 0 | 0 0 0 | 0 0 0 |
| IR8-1 (3) | 0 1 0 | 0 −1 0 | 0 −1 0 | 0 1 0 | 0 0 0 | 0 0 0 | 0 0 0 | 0 0 0 | 0 0 0 | 0 0 0 | 0 0 0 | 0 0 0 |
| | 0 0 1 | 0 0 1 | 0 0 1 | 0 0 1 | 0 0 0 | 0 0 0 | 0 0 0 | 0 0 0 | 0 0 0 | 0 0 0 | 0 0 0 | 0 0 0 |
| | 0 0 0 | 0 0 0 | 0 0 0 | 0 0 0 | 0 0 0 | 0 0 0 | 0 0 0 | 0 0 0 | 0 0 1 0 | 0 0 1 | 0 0 1 | 0 0 1 |
| IR8-2 (3) | 0 0 0 | 0 0 0 | 0 0 0 | 0 0 0 | 0 0 1 0 | 0 0 1 | 0 0 1 | 0 0 1 | 0 0 0 | 0 0 0 | 0 0 0 | 0 0 0 |
| | 0 0 0 | 0 0 0 | 0 0 0 | 0 0 0 | 1 0 0 | −1 0 0 | −1 0 0 | 1 0 0 | 0 0 0 | 0 0 0 | 0 0 0 | 0 0 0 |
| | 0 0 0 | 0 0 0 | 0 0 0 | 0 0 0 | 0 0 1 0 | 0 0 −1 | 0 0 −1 | 0 0 1 | 0 0 0 | 0 0 0 | 0 0 0 | 0 0 0 |
| IR8-3 (3) | 0 0 0 | 0 0 0 | 0 0 0 | 0 0 0 | 1 0 0 | 1 0 0 | 1 0 0 | 1 0 0 | 0 0 0 | 0 0 0 | 0 0 0 | 0 0 0 |
| | 1 0 0 | 1 0 0 | 1 0 0 | 1 0 0 | 0 0 0 | 0 0 0 | 0 0 0 | 0 0 0 | 0 0 0 | 0 0 0 | 0 0 0 | 0 0 0 |
| | 0 0 0 | 0 0 0 | 0 0 0 | 0 0 0 | 0 0 0 | 0 0 0 | 0 0 0 | 0 0 0 | 1 0 0 | 1 0 0 | 1 0 0 | 1 0 0 |
| IR8-4 (3) | 0 0 0 | 0 0 0 | 0 0 0 | 0 0 0 | 0 0 0 | 0 0 0 | 0 0 0 | 0 0 0 | 0 1 0 | 0 −1 0 | 0 −1 0 | 0 1 0 |
| | 0 0 0 | 0 0 0 | 0 0 0 | 0 0 0 | 0 0 0 | 0 0 0 | 0 0 0 | 0 0 0 | 1 0 0 | −1 0 0 | −1 0 0 | 1 0 0 |
| | 0 0 0 | 0 0 0 | 0 0 0 | 0 0 0 | 0 0 0 | 0 0 0 | 0 0 0 | 0 0 0 | 0 0 1 | 0 0 −1 | 0 0 −1 | 0 0 1 |
| IR8-5 (3) | 0 0 0 | 0 0 0 | 0 0 0 | 0 0 0 | 0 1 0 | 0 1 0 | 0 1 0 | 0 1 0 | 0 0 0 | 0 0 0 | 0 0 0 | 0 0 0 |
| | 0 1 0 | 0 1 0 | 0 1 0 | 0 1 0 | 0 0 0 | 0 0 0 | 0 0 0 | 0 0 0 | 0 0 0 | 0 0 0 | 0 0 0 | 0 0 0 |
| | 0 0 1 | 0 0 −1 | 0 0 −1 | 0 0 1 | 0 0 0 | 0 0 0 | 0 0 0 | 0 0 0 | 0 0 0 | 0 0 0 | 0 0 0 | 0 0 0 |

TABLE S6. List of the coordinates of Tb atoms in a unit cell. The rest of the half atoms are induced by centering symmetry +(1/2, 1/2, 1/2)

| | | | |
|---|---|---|---|
| Tb1 | 0 | $y$ | $z$ |
| Tb2 | 0 | $-y+1$ | $z$ |
| Tb3 | 0 | $y$ | $-z+1$ |
| Tb4 | 0 | $-y+1$ | $-z+1$ |
| Tb5 | $z$ | 0 | $y$ |
| Tb6 | $z$ | 0 | $-y+1$ |
| Tb7 | $-z+1$ | 0 | $y$ |
| Tb8 | $-z+1$ | 0 | $-y+1$ |
| Tb9 | $y$ | $z$ | 0 |
| Tb10 | $-y+1$ | $z$ | 0 |
| Tb11 | $y$ | $-z+1$ | 0 |
| Tb12 | $-y+1$ | $-z+1$ | 0 |
